# Supplementary material for: Unifying Regularisation Methods for Continual Learning
Source: arXiv:2006.06357 source file (2021-02-03)
Supplement: Supplementary file 1 [file 00_overview.tex]

\section{APPENDIX}
\tableofcontents
\iffalse
This appendix has several components:
\begin{enumerate}
	\item A tabular overview over algorithms and baselines described in the paper, \ref{sec:tabular_overview}
	\item Full experimental details including hyperparameter seraches and values, as well as full details about Batch-EF,  Appendix \ref{sec:exp_detail}. 
	\item Performance and Relation to Fisher of MAS based on logits, Appendix \ref{sec:MAS_logits}
	\item Two improvements of SI, Apprendix \ref{sec:late_SI}
	\item A more detailed account of the influence of the optimizer on SI, Apprendix \ref{sec:SI_optimizer}.
	\item Details for two calculations omitted in the main paper, Appendix \ref{sec:SI-OnAF-calc}. 
	%We give the details of two calculations omiited in our derivation that SI and AF are related, see Appendix \ref{sec:calc}
	\item We empirically investigate the gradient noise in Appendix \ref{sec:noise}. This experiment is not specific to continual learning.
	%\item  We provide an empirical comparison of different versions of the Fisher Information (`real', `empirical' and `predicted') in Appendix \ref{sec:fishers}.
		%\item We provide a short interpretations of why the Absolute Fisher can be interpreted as a justified importance measure in Appendix \ref{sec:th_abs_fish}. 
	\item We critically review experimental claims from previous work about regularisation methods in Appendix \ref{sec:reg}. 
	%\item We describe some variants of SI and OnAF, which we tried with the aim of improving performance in Appendix \ref{sec:SI_variants}.
	\item We include additional experiments and plots in Appendix \ref{moreisbetter}, including investigations how rescaling SI affects its relation to AF.
	%We show plots analogous to the ones from the main paper, but evaluated on datasets/tasks not shown in the main paper. This highlights the effect that the regularisation term in the loss function has on SI. It shows that strong regularisation weakens SI's relation to OnAF, c.f. Section \ref{sec:all_plots}. 
\end{enumerate}\fi
