# Supplementary material for: Unifying Regularisation Methods for Continual Learning
Source: arXiv:2006.06357 source file (2021-02-03)
Supplement: Supplementary file 2 [file SI_optimizer.tex]

\section{Influence of Optimizer on SI}\label{sec:SI_optimizer}
	As pointed out in the main paper, the bias of SI depends on the optimizer used. For SGD+momentum, one can follow precisely the same steps as for Adam (simply ignoring the division by its second moment estimate) to see that in this case SI will resemble the Online Fisher, i.e. (assuming a learning rate of $1.0$)
	$$
	\tilde{\omega}(SI)\approx (1-\beta_1)\sum_t (g_t +\sigma_t)^2
	$$
	Analogously to Adam, in this case the relation of SI to the Fisher is due to the bias of SI. 
	Thus, checking whether in this situation, too, the unbiased version SIU performs worse than SI, is another validation of our theory. Indeed, on P-MINST, we found that SI with SGD and momentum achieves an average of $97.4\%$, while the best run for SIU was at $96.1\%$. We did not test SGD further, due to instabilities described now:
	For both SI, SIU using SGD+momentum resulted in unstable behaviour, with runs occasionally diverging. This is likely due to the fact the the regularisation loss is ill-conditioned, since the importances span several orders of magnitudes. This suggests that, without further tricks and efforts, adaptive optimisers are a more suitable choice for regularisation methods. 
	
For other ootmisers, the bias of SI will take different shapes and how this affects performance will have to be seen. Our theory suggests, that biasing SI to (a version of) the Fisher will help its performance, while we predict that fundamentally different biases lead to SI having worse performance than e.g.\ OnAF. An instructive example in this case is considering an approximation of natural gradient descent, which preconditions with the inverse diagonal of the empirical fisher (rather than the inverse fisher, which is expensive to compute). In this case, SI would have constant importances (across parameters) and would likely perform badly.
