# Supplementary material for: Unifying Regularisation Methods for Continual Learning
Source: arXiv:2006.06357 source file (2021-02-03)
Supplement: Supplementary file 3 [file abs_fish.tex]

\section{A theoretical Interpretation of Fisher and Absolute Fisher}\label{sec:th_abs_fish}
Here, we briefly explain how the Absolute Fisher can be seen as a principled importance measure, beyond the fact that it is highly correlated with the Fisher Information (which could already be reason enough to think it effective).
We first review the Bayesian motivation of EWC to use the Fisher Information \citep{kirkpatrick2017, huszar2018} and point out a frequentist interpreation of the same idea. The frequentist interpretation is somewhat immediate, the first written account we are aware of is presented in \cite{yin2020sola}.

\subsection{Fisher from a Bayesian Perspective}
Assume for simplicity that we want to learn only two datasets $\mathcal{D}_A,\mathcal{D}_B$ sequentially. We either write $(X,y)\sim \mathcal{D}_A$ for a sample from $\mathcal{D_A}$ consisting of an input $X$ and its label $y$, or we will slightly abuse notation and write $X\sim \mathcal{D_A}$ for a sample of an input only.

Taking a bayesian perspective, we eventually would like to find $p(\theta\mid \mathcal{D}_A, \mathcal{D}_A)$. During training, we do not have access to both sets simultaneously, but we can rewrite our objective as 
\begin{eqnarray*}
\log p(\theta\mid \mathcal{D}_A, \mathcal{D}_B) &=& \log p(\theta \mid \mathcal{D}_A) + \log p(\mathcal{D}_B\mid \theta, \mathcal{D}_A) - \log p(\mathcal{D}_B \mid \mathcal{D}_A) \\
&=& \log p(\theta \mid \mathcal{D}_A) + \log p(\mathcal{D}_B\mid \theta) - \log p(\mathcal{D}_B \mid \mathcal{D}_A),
\end{eqnarray*}
For optimizing this objective w.r.t.\ $\theta$, we do not need to evaluate the third term of this sum. The second term is the standard loss that we optimize during training on dataset $B$. The first term is generally intractable and the idea of EWC is to use a second-order Taylor approximation of $\log p(\theta \mid \mathcal{D}_A)$ around $\theta_A$, which denotes the point estimate of $\theta$ obtained after training on the first task. To spell out the Taylor expansion, denote the Hessian of $\log p(\theta_A \mid \mathcal{D}_A)$ w.r.t.\ $\theta$ by $H_A$ and note that $\nabla_\theta \log p(\theta_A \mid \mathcal{D}_A)\approx 0$, since we have minimised this term w.r.t.\ $\theta_A$ and hopefully found a local minimum. We thus obtain 
$$
\log p(\theta\mid \mathcal{D}_A, \mathcal{D}_B) \approx (\theta-\theta_A)^T H_A (\theta-\theta_A)+ \log(\mathcal{D}_B\mid \theta) + \text{constant}
$$
This is the training objective proposed by EWC, which first approximates $H_A$ by the Fisher Information and then approximates the Fisher Information by its diagonal. The advantage of the Fisher $F$ is that it is cheap to compute and that it is positive semi-definite. It is a principled approximation of the Hessian $H_A$ in the following sense (see below for justifications of each equation):
\begin{eqnarray}
-F &=& \frac{\partial^2 }{\partial \theta^2}\EE_{X\sim \mathcal{D_A}}\EE_{y\sim p_X}[\log p_X(y)] \label{eq1}\\
&\approx& \frac{\partial^2 }{\partial \theta^2}\EE_{(X,y)\sim \mathcal{D_A}}[\log p_X(y)] \label{eq2}\\
&=& \frac{1}{N} \frac{\partial^2 }{\partial \theta^2} \log p(\mathcal{D}_A\mid \theta) \label{eq3}\\
&\approx & \frac{1}{N} \frac{\partial^2 }{\partial \theta^2} \log p(\theta \mid \mathcal{D}_A) \label{eq4} \\
&=&\frac{1}{N} H_A \label{eq5}
\end{eqnarray}
The equality \eqref{eq1} is obtained from basic algebraic manipulations, see e.g.\ appendix of \cite{pascanu2013revisiting}. The approximation \eqref{eq2} comes from assuming that the model learned to nearly perfectly classify all inputs. The equality \eqref{eq3} is immediate, $N$ denotes the number of datapoints in our (empirical) distribution $\mathcal{D}_A$. The approximation \eqref{eq4} takes the second derivative of 
$ \log p(\mathcal{D}_A \mid \theta) = \log p(\theta \mid \mathcal{D}_A)  - \log p(\theta) + \log p(\mathcal{D}_A)$ and ignores the term stemming from the prior $p(\theta)$, which is justified in the infinite data limit. The last equation \eqref{eq5} is by definition of $H_A$.

\subsection{Fisher from a Frequentist Perspective}
The frequentist interpretation of the Fisher assumes that we aim to minimize the negative log-likelihood of the data for each of our tasks. 

As explained above (recall equations \eqref{eq1}-\eqref{eq3}), the Fisher Information is  an approximation of the Hessian of $\log p(\mathcal{D_A} \mid \theta)$ w.r.t. $\theta$. Denoting again by $\theta_A$ the parameters obtained after training the first task, we can approximate the loss (negative log-likelihood) on the first task around $\theta_A$ using a Taylor approximation to obtain (noting that close to a local minimum $\theta_A$ we have $\nabla_\theta p(\mathcal{D}_A\mid \theta)\approx 0$)
\begin{eqnarray*}
-\log p(\mathcal{D}_A)
&\approx& \text{constant} + (\theta-\theta_A)^T \nabla_\theta p(\mathcal{D}_A \mid \theta) + (\theta-\theta_A)^T F (\theta-\theta_A)  \\
&\approx& \text{constant} + (\theta-\theta_A)^T F (\theta-\theta_A)
\end{eqnarray*}
Recall that the loss of EWC when training on dataset $\mathcal{D}_B$ is
$$
\log(p(\mathcal{D}_B)) + \lambda \cdot (\theta_A)^T F (\theta_A)
$$
As explained above, minimizing the second term in this sum is approximately equivalent to minimising the negative log-likelihood of the data $\mathcal{D}_A$. Thus, the objective of EWC is to jointly optimize the log-likelihood of both datasets.

\subsection{Theoretical Interpretation of Absolute Fisher}
Here, we present a frequentist interpretation of the Absolute Fisher for continual learning, which is analogous to the frequentist interpretation of using the Fisher Information (and which assumes knowledge of the latter).

Write AF for the Absolute Fisher and note that
\begin{eqnarray}
\text{AF} &=& \frac{\partial^2 }{\partial \theta^2}\EE_{X\sim \mathcal{D_A}}\EE_{y\sim p_X}[\log p_X(y)] \label{eq1}\\
&\approx& \frac{\partial^2 }{\partial \theta^2}\EE_{(X,y)\sim \mathcal{D_A}}[\log p_X(y)] \label{eq2}\\
&=& \frac{1}{N} \frac{\partial^2 }{\partial \theta^2} \log p(\mathcal{D}_A\mid \theta) \label{eq3}\\
&\approx & \frac{1}{N} \frac{\partial^2 }{\partial \theta^2} \log p(\theta \mid \mathcal{D}_A) \label{eq4} \\
&=&\frac{1}{N} H_A \label{eq5}
\end{eqnarray}

\EE

The frequentist interpretation of the Fisher was based on the choice of optimizing log-likelihood. This choice fits well into several theoretical frameworks and simplifies many calculations. However, eventually, if we care about performance measures such as classification accuracy, it remains a surrogate to our real objective. If we replace this surrogate by a different one (i.e.\ if we choose a different loss function) and then use a Taylor expansion to approximate this loss function we will recover the Absolute Fisher rather than the Fisher:

Let's consider the following alternative loss function
$$\EE_{(X,y)\sim \mathcal D}\left[ \left(p((X,y)\mid\theta)-1\right)\cdot \log p((X,y)\mid\theta)\right].$$ 
Note that this loss, just like the negative log-likelihood, is monotone in the likelihood (for each individual datapoint) and is 0 if and only if all inputs are classified perfectly. 
Calculating the Hessian of this loss gives
\begin{eqnarray}
\frac{\partial^2}{\partial \theta^2} \EE_{X\sim \mathcal D}\left[ \left(p((X,y)\mid\theta)-1\right)\cdot \log p((X,y)\mid\theta)\right] \\
= \frac{\partial^2 \p}{\partial \theta^2} \log a
\end{eqnarray}
