# Supplementary material for: Unifying Regularisation Methods for Continual Learning
Source: arXiv:2006.06357 source file (2021-02-03)
Supplement: Supplementary file 4 [file variants.tex]

\section{Variants of SI/OnAF}\label{sec:SI_variants}
Based on our findings, we investigated several adoptions of SI as described below. 

Firstly, rather than taking the running sum of the product of gradient and update for SI, we experimented with an exponential moving average (EMA). We tried this based on our evidence that SI approximates some form of the Fisher Information. The EMA puts more weight on recently observed samples of this value, which should be more related to the actual Fisher Information and discards information which stems too far from the past. We performed HP searches over different decay factors for the running average on P-MNIST and found small improvements. Additionally, we found that the EMA is less stable if training time is increased (to e.g.\ 100 or 200 epochs per task). In this case, the magnitude of the EMA after for example the first task varies greatly from run to run (since the parameters may or may not be in a very flat region of the loss landscape), while the running sum (as in SI) is more stable (as we observed empirically).

Secondly, observe that the magnitude of the per-task-importance of SI depends largely on how long we train, rather than on the change in loss. This can be seen for examples in Figure \ref{figure:summed_cifar_all}, where the importances of the CIFAR 100 tasks are considerably smaller than the importance of the CIFAR 10 task. This is partly because each class in CIFAR 100 has 10 times less training samples, corresponding to 10 times less training iterations when keeping the number of epochs fixed (at 60 in our case). This suggests rescaling the per-task-importance by the number of training iterations of that task. We simply divided the importance of each task by the number of training iterations of that task (and performed a new HP search). We found no change in performance with this rescaling.

Thirdly, recall that we argued that SI is closely related to the running sum of absolute gradient values, OnAF. We also implemented an importance measure based on 
the running sum of squared gradients (OnF -- Online Fisher), as this variant more closely matches the Real Fisher Information. We observed a slight decrease in performance. 

We believe that our findings may indicate that regularisation based continual learning is fairly robust to rescaling its importance measures, at least on the datasets/settings we tested.
