# Supplementary material for: Unifying Regularisation Methods for Continual Learning
Source: arXiv:2006.06357 source file (2021-02-03)
Supplement: Supplementary file 5 [file X_B_SI-AF.tex]

\section{Synaptic Intelligence approximates (Online) Absolute Fisher}
Here, we explain why the importance measure of SI is related to the Absolute Fisher, despite the apparent contrast between SI's path integral and the Fisher Information. The theoretical part first identifies the bias that SI introduces when approximating the path integral. It then relates the bias to the Absolute Fisher. As before, we carefully validate each theoretical argument empirically.

%\subsection{Theoretical Relation of SI and Absolute Fisher}
\subsection{Bias of Synaptic Intelligence}\label{bias}
To calculate $\omega(\SI)$ (see \eqref{eq:def_SI}), we need to calculate the product $p = \frac{\partial L(t)}{\partial \theta}\cdot\Delta(t)$ at each step $t$. Since evaluating the full gradient $\frac{\partial L(t)}{\partial \theta}$ is prohibitively expensive, SI \citep{zenke2017} uses a stochastic mini-batch gradient. The resulting estimate is biased since the same mini-batch is used for the parameter update $\Delta(t)$ and the estimate of $\frac{\partial L(t)}{\partial \theta}$. 

We now give the calculations detailing the argument above.
For ease of exposition, let us assume that the network is optimized using vanilla SGD with learning rate $1$. 
%Very similar arguments apply to other optimizers. 
Given a mini-batch, denote its gradient estimate by $g+\sigma$, where $g=\frac{\partial L(t)}{\partial \theta}$ denotes the real gradient and $\sigma$ the mini-batch noise. The parameter update equals $\Delta(t) =  g+\sigma$. Thus, our product $p$ should be  
$p = g \cdot(g+\sigma).$ 
However, using $g+\sigma$, which was used for the parameter update, to estimate $\frac{\partial L(t)}{\partial \theta_i}$ results in 
$p_{biased} = (g+\sigma)^2.$ 
Thus, the gradient noise introduces a bias of
$\mathbb{E}[\sigma^2 +\sigma g] = \EE[\sigma^2].$

\paragraph{Unbiased Synaptic Intelligence.}
Having understood the bias, we can design an unbiased estimate by using two independent mini-batches to calculate the parameter update and to estimate $g$. This way we get $\Delta(t) =  g+\sigma$ and an estimate $g+\sigma'$ for $g$ from an independent mini-batch with independent noise $\sigma'$. We obtain
$
p_{unbiased} = (g+\sigma') \cdot (g+\sigma) 
$
which in expectation equals $p = g \cdot(g+\sigma).$
Based on this we define an unbiased importance measure
$$
\tilde{\omega_i}(\SIU) =  \sum_{t=0}^{T-1} (g_t+\sigma_t') \cdot \Delta(t). 
$$
%where the dash indicated that the gradient estimate is independent of the parameter update.

\paragraph{Bias-Only version of SI.}\label{bias_only}
To isolate the bias, we can take the difference between biased and unbiased estimate. Concretely, this gives an importance which only measures the bias of SI %and is independent of the path integral, 
$$
\tilde{\omega_i}(\SIB) =   \sum_{t=0}^{T-1} ((g+\sigma)-(g+\sigma_t')) \cdot \Delta(t). 
$$ Observe that this estimate multiplies the parameter-update $\Delta(t)$ with nothing but stochastic gradient noise. From the perspective of the SI path-integral, this should be meaningless and perform poorly.

\subsection{Relation of Bias of SI to Absolute Fisher}\label{sec:SI_FI}
The bias of SI found above depends on the optimizer used. The original SI-paper (and we) uses Adam \citep{kingma2014adam}. A detailed derivation of the effect of Adam on the bias is given in Appendix \ref{sec:SI-OnAF}. Here, we summarise the main result as well as testable assumptions and predictions given by our derivation (empirical confirmations are deferred to next section): 
We find that with Adam SI approximates the (Empirical) Online Absolute Fisher, c.f.\ Table \ref{table:overview}. 
The derivation mainly relies on the bias of SI (directly linked to gradient noise) being larger than the unbiased part. Moreover, the derivation predicts that the relation between SI and OnAF gets weaker as the influence of the regularisation loss on parameter updates increases. Additionally, we find that in the presence of large gradient noise, the Empirical Fisher can be evaluated in mini-batches and use these insights to develop and test a faster version of the EWC algorithm.

OnAF can be seen as averaging AF along the parameter trajectory during training, raising the question how similar these two measures are. 
%It is not a priori clear whether this average or the final point estimate will turn out more useful for continual learning, since the parameters move away from the final point as soon as a new task arrives. It is also not obvious, how closely related OnAF and AF are. 
The fact that across a huge number of deep learning settings, the second moment estimate of Adam uses a rather slowly decaying exponential average ($\beta_2=0.999$) suggests that in many settings the second moment changes very slowly along the parameter trajectory. Intriguingly, this second moment is almost the same as the AF (where only the square is replaced by an absolute value), so that we hypothesise that OnAF and AF are closely related (as AF changes slowly along the parameter trajectory). Since SI is related to OnAF, this leads to our claim that SI (like MAS) approximates AF.

\subsection{Emprical Investigation of SI, its bias and Absolute Fisher}
%Our first important insight was recognising the bias of SI, which we now investigate empirically.

\textbf{Magnitude of Bias.} Note that according to the motivation of SI (see \eqref{def_contribution}) the sum of its importances should track the decrease in loss $L(0)-L(T)$. Therefore, we tracked the summed importances for SI and its unbiased version SIU during training. As a control we also included an approximation of the path integral based on the full training gradient (rather than approximating it). The results in Figure \ref{figure:SI} (left) show several things:  (1) the bias is 5-6 times larger than the unbiased part;  (2) using an unbiased gradient estimate and using the entire training set gradient gives almost identical values of $\sum_i\omega_i$ supporting the validity of the unbiased estimator; (3) even the unbiased first order approximation of the path integral overestimates the decrease in loss. This is consistent with previous empirical studies showing that the loss has positive curvature \citep{jastrzebski2018relation, lan2019}.  
%Note that the large magnitude of the bias (i.e.\ the noise) also shows that our approximation in eq \eqref{eq:noise} is valid, see \ref{sec:calc_bias} for full details. 
Additionaly, since the bias is caused by gradient noise, we performed a more detailed analysis of the noise in Appendix \ref{sec:noise} finding further support for our claims and derviations.

\textbf{Bias and Performance.} Above we saw that the bias is considerably larger than the unbiased part. But how does it influence SI's performance? To quantify this, we ran continual learning algorithms using the importance measure of SI, its unbiased version SIU and the bias-only version SIB. Note that SIB is completely independent of the path integral motivating SI, only measures gradient noise and therefore should perform poorly from the perspective of SI. However, our empirical results in Table \ref{table:results}(2), reveal the opposite: Removing the bias reduces performance of SI (SIU is worse), whereas isolating the bias does not affect or slightly improves performance. This is very strong evidence for the claim that SI relies on its bias for its continual learning performance. 

\textbf{Bias and Fisher.} As additional experiment, we checked how much the relation of SI to the Fisher depends on the bias. Our theory predicts that the relation between SI and the Online Absolute Fisher (OnAF) is mostly based on the bias (see \ref{sec:calc_bias}). Figure \ref{figure:SI} (mid) confirms this, showing a strong correlation between SI, SIB and OnAF and a weaker correlation between SIU and OnAF as expected. 
%Note that this also shows that eq \eqref{eq:SI-OnAF} is valid.

In summary, the bias dominates SI and causes both its performance and its relation to OnAF. %This supports our claim that SI works because it approximates OnAF.

\textbf{Relation of SI \& OnAF to AF.} Next, we investigated the relation between OnAF and AF, finding  strong correlations between the two (between 0.73-0.87 on MNIST and 0.86-0.95 on CIFAR). Figure \ref{figure:SI} shows that this relation directly carries over to relating SI and AF. An additional control in \ref{sec:training_time} shows that this is not an artefact of long training times. 
These results empirically substantiate our derivation that SI is closely related to the Absolute Fisher. 
\begin{wrapfigure}[15]{r}{0.4\textwidth}
	%\vskip -0.25in
	\begin{center}
		\includegraphics[width=0.38\textwidth]{../figures/time_mnist_log.png}
	\end{center}
	\vskip -0.02in
	\caption{Wall-Clock Time (log sale) for EWC and new versions measured on P-MNIST. Batch-EF (ours) approximates the Fisher more than 800x faster.}
	\label{figure:time}
	%\vskip -0.15in
\end{wrapfigure}

\textbf{Effect of Regularisation on SI.} Lastly, we assesed our prediction that large regularisation will diminish the correlation between SI and OnAF, by comparing standard SI to two variants of with less strong regularisation. The first control simply sets regularisation strength to $c=0$. The second control refrains from re-initialising the network weights after each task (exactly as in the original SI paper, albeit with slightly worse validation performance). In the second setting the current parameters $\theta$ never move too far from their old value $\theta^{(k-1)}$, implying smaller gradients from the quadratic regularisation loss, and also meaning that a smaller value of $c=0.5$ is optimal. We see that for both controls with weak regularisation the relation to OnAF is larger than for standard-SI with strong regularisation (Figure \ref{figure:SI} (right)), verifying our prediction.

\textbf{Efficient version of EWC.} Our derivation (see \ref{sec:SI-OnAF} for full details) shows that the Fisher can be approximated by the Empirical Fisher and that the gradient computation for the Empirical Fisher can be averaged across mini-batches (before it is squared) rather than carried out for each image individually. This is important as it offers large computational savings. First, we checked that the approximations described above do not harm performance. To this end we evaluated EWC (using the `real' Fisher) and compared it to a variant using the Empirical Fisher and a variant calculating the Empirical Fisher in mini-batches (Batch-EF), c.f.\ \ref{sec:ewc_details}. The results (Table \ref{table:results} (4)) show that the approximations have the same performance as EWC. At the same time, our final algorithm Batch-EF is more than 800x faster than EWC at approximating the Fisher (Figure \ref{figure:time}); on Split CIFAR the speed up is >300x. Moreover, note that EWC is dominated by the time it needs to approximate the Fisher, while for our sped-up Batch-EF this is negligible and total time is dominated by training time.

\begin{figure}[t]
	\begin{center}
		\begin{subfigure}{0.32\textwidth}
			%\vskip 0.1in
			\centerline{\includegraphics[width=\textwidth]{../figures/summed_contributions_MNIST.png}}
		\end{subfigure}
		\begin{subfigure}{0.3\textwidth}
			%\vskip 0.1in
			\centerline{\includegraphics[width=\textwidth]{../figures/correlations_MNIST_bias.png}}
		\end{subfigure}
		\begin{subfigure}{0.3\textwidth}
			%\vskip 0.1in
			\centerline{\includegraphics[width=\textwidth]{../figures/correlations_CIFAR_SI_reg.png}}
		\end{subfigure}
	\end{center}
		\caption{\textbf{Effect of Bias and Regularisation on SI.}
			\textit{Left:} Summed Importances for SI and its unbiased version on MNIST, showing that the bias dominates SI. 
			\textit{Mid:} Pearson Correlations of SI, its bias (SIB), and unbiased version (SIU) on MNIST, showing that relation between SI and (On)AF is due to bias.
			\textit{Right:} Relation between SI and OnAF and two SI-controls: `$c=0$' has regularisation strength $0$; `no re-init' does not re-initialise network weights after each task. This shows that strong regularisation weakens the tie between SI and (On)AF as predicted.
		}
		\label{figure:SI}
	\vskip -0.15in
\end{figure}
