# Supplementary material for: Unifying Regularisation Methods for Continual Learning
Source: arXiv:2006.06357 source file (2021-02-03)
Supplement: Supplementary file 6 [file SI_AF.tex]

\section{Detailed Calculations for the bias of SI, and for calculating Fisher in Batches}\label{sec:SI-OnAF-calc}
Here we give the details for two calculations omitted in the main text.
\subsection{Formula of Bias of SI with Adam}\label{sec:calc_bias}
Here, we show that the bias, i.e.\ the expected difference between SI and SIU, is equal to $(1-\beta_1)\sigma_t^2/(\sqrt{v_t}+\epsilon)$ and that Assumption 1 is equivalent to the bias being larger than the unbiased part of SI. 

Recall that for SI, we approximate  $\frac{\partial L(t)}{\partial \theta}$ by $g_t+\sigma_t$, which is the same gradient estimate given to Adam. So we get
\begin{align*}
\textbf{SI:}&\qquad \frac{\partial L(t)}{\partial \theta} \Delta(t) = 
%(g+\sigma)\cdot \frac{(1-\beta_1)(g+\sigma) + \beta_1 m_{t-1}}{\sqrt{v_t} + \epsilon} \\
\frac{(1-\beta_1)(g_t+\sigma_t)^2}{{\sqrt{v_t} + \epsilon}} + \frac{\beta_1(g_t+\sigma_t)m_{t-1}}{{\sqrt{v_t} + \epsilon}}.\\
\intertext{For SIU, we use an independent mini-batch estimate $g_t+\sigma'_t$ for $\frac{\partial L(t)}{\partial \theta}$ and therefore obtain
} 
%\begin{eqnarray*}
\textbf{SIU:}&\qquad \frac{\partial L(t)}{\partial \theta} \Delta(t) =
%(g+\sigma)\cdot \frac{(1-\beta_1)(g+\sigma) + \beta_1 m_{t-1}}{\sqrt{v_t} + \epsilon} \\
\frac{(1-\beta_1)(g_t+\sigma'_t)(g_t+\sigma_t)}{{\sqrt{v_t} + \epsilon}} + \frac{\beta_1(g_t+\sigma'_t)m_{t-1}}{{\sqrt{v_t} + \epsilon}}.\\
\intertext{Taking the difference between these two and ignoring all terms which have expectation zero (note that $\EE[\sigma_t]=\EE[\sigma'_t] = 0$ and that $\sigma_t, \sigma'_t$ are independent of $m_{t-1}$ and $g_t$) gives
}
\textbf{SI}-\textbf{SIU:}&\qquad (1-\beta_1)\frac{\sigma_t^2}{\sqrt{v_t}+\epsilon}
\end{align*}
as claimed.

To see that Assumption 1 is equivalent to the bias being larger than the unbiased part, note that in expectation SIU equals $$(1-\beta_1)\frac{g_t^2}{\sqrt{v_t}+\epsilon} + \beta_1\frac{g_t m_{t-1}}{\sqrt{v_t}+\epsilon}\approx \beta_1\frac{m_{t-1} g_t}{\sqrt{v_t}+\epsilon} $$
The last approximation here is valid because $\beta_1m_{t-1}\gg (1-\beta_1)g_t$ which holds since (1) $\beta_1 \gg (1-\beta_1)$ and (2) $\EE[|m_{t-1}|]\ge\EE[|g_t|]$. (1) follows from $\beta_1=0.9$, and (2) holds since $\EE[m_{t-1}]\approx g_t$ and since $m_{t-1}$ has a noise component (due to gradient noise), while $g_t$ is a deterministic quantity, implying $\EE[|m_{t-1}|]\ge\EE[|g_t|]$ by elementary considerations.

In particular, the two calculations for the bias and the expectation of SIU above imply that Assumption 1, which is $(1-\beta_1)\sigma_t^2 \gg \beta_1 m_{t-1} g_t$, is equivalent to the bias of SI being larger than its unbiased part. 

\subsection{Effect of Calculating Fisher in Mini-Batches: Analysis of Batch-EF}\label{sec:calc_batch}
For this subsection, let us slightly change notation and denote the images by $X_1,\ldots, X_D$ and the gradients (with respect to their labels and the cross entropy loss) by $g+\sigma_1, \ldots g+\sigma_D$. Here, again $g$ is the overall training set gradient and $\sigma_i$ is the noise (i.e.\ $\sum_{i=1}^{D} \sigma_i = 0$). Then the Empirical Fisher is given by 
\[
\text{EF} = \frac{1}{D}\sum_{i=1}^D (g+\sigma_i)^2 
\] 
We want to compare this to evaluating the squared gradient over a batch. Let $i_1, \ldots, i_b$ denote uniformly random, independent indices from $\{1,\ldots, D\}$, so that $X_{i_1}, \ldots, X_{i_b}$ is a random mini-batch of size $b$. Let $g+\sigma$ be the gradient on this mini-batch. We then have, taking expectations over the random indices, 
\begin{eqnarray*}
	\EE[(g+\sigma)^2] &=& \EE\left[ \frac{1}{b^2}\sum_{r,s=1}^b (g+\sigma_{i_r})(g+\sigma_{i_s})\right] \\
	&=& \frac{b(b-1)}{b^2} \EE[(g+\sigma_{i_1})(g+\sigma_{i_2})]  +\frac{b}{b^2}\EE[(g + \sigma_{i_1})^2]\\
	&=& \frac{b-1}{b} g^2 + \frac{1}{b} \text{EF}\\
	&\approx& \frac{1}{b} \text{EF}
\end{eqnarray*}
This conclusion may seem surprising, but recall that it is only based on one assumption, namely that the gradient noise is considerably bigger than the gradient itself - an assumption for which we have collected ample evidence. 

This conclusion may seem surprising, but it only relies on only two assumptions: (1) We draw a minibatch with i.i.d.\ elements (i.e.\ with replacement) , and (2) the noise is considerably bigger than the gradient.

(1) If we draw minibatch elements without replacement (on the extreme end would be drawing the full batch), then our derivation ignores the contribution of $\EE[\sigma_{i_1}\sigma_{i_2}]<0$. Note that as long as the batchsize is small (square root of the size of the dataset or smaller) drawing a batch with or without replacement has almost the same distribution.

(2) Concretely, we assume $\EE[(g+\sigma_i)^2]\gg (b-1) g^2$. Note that unlike in other sections of this manuscript, here $\sigma_i$ refers to the gradient noise of individual images (rather than mini-batch noise). We have seen that even with a batch-size of 256 (i.e.\ when we reduce then noise by a factor of 256) the noise is still much bigger than the gradient (recall Figures \ref{figure:summed_mnist_all}, \ref{figure:summed_cifar_all}, \ref{figure:noise}, \ref{figure:noise_cdf}), so that our assumption is true with room to spare.

We also point out that the relation between the (diagonal of the) covariance matrix of minibatch gradients and the Fisher Information has also been described in several other places in the literature, e.g.\ \cite{roux2008topmoumoute, thomas2020interplay, jastrzkebski2017three}.

%We also mention preliminary and unsurprising experiments, in which we evaluated the Empirical Fisher in mini-batches on P-MNIST (at the end of training a task) and observed the same performance as when evaluating the Empirical Fisher (and also `real' Fisher) on single images.
