# Supplementary material for: Unifying Regularisation Methods for Continual Learning
Source: arXiv:2006.06357 source file (2021-02-03)
Supplement: Supplementary file 7 [file late_SI.tex]

\section{Improvements of SI}\label{sec:late_SI}
	As we have argued in the discussion, we expect SI to be a more faithful approximation of AF if more weight is put on the summands of SI (see \eqref{eq:def_SI}), which occur later in training. As a consequence, putting more weight on latter summands could lead to better performance. We tested this prediction by running two variants of SI. For the first one, we only considered summands occuring in the second half of training (epochs 10 to 20, of 20). For the second one, we used an exponential moving average with a deacy of $0.999$. Both variants achieved an average accuracy on P-MNIST of $97.5\%$, which is better than SI's $97.2\%$. This confirms our prediction.
